# Supplementary material for: Mixed H2/H-infinity Data-Driven Control Design for Hard Disk Drives
Source: arXiv:1804.03298 source file (2018-04-10)
Supplement: Supplementary file 1 [file 7-Appendix.tex]

%\appendix

\subsection{Proof of Theorem~\ref{THEOREMMISOHINF}}\label{ch:Appendix:Proof}
\input{7-Appendix/7-Appendix_Proof}

\subsection{The $H_\infty$ constraints}\label{ch:Appendix:HinfResults}
\input{7-Appendix/7-Appendix_Hinf}
